# Supplementary material for: An Empirical Study of Refactoring Engine Bugs
Source: arXiv:2409.14610 source file (2024-09-22)
Supplement: Supplementary file 1 [file appendix.tex]

This means most of our finding simplifications are refactoring, developers in OSS have already tried to debloating code by using refactoring, which aligns with existing researches~\cite{sharif2018trimmer,kalhauge2021logical}. For example, extracting method is one of the most common program refactoring type that also result in simplified program. In listing~\ref{lst:extract_method_example}, both methods in line 5 and line 12 check whether a String object is empty, it is very obvious that those code blocks are duplicated and can be extracted out as a single method. A short and well-named method called \texttt{isEmpty} is created, thus it can be reused in any place for checking empty.
\begin{lstlisting}[style=mystyle, escapechar=^,caption=Example of extracting method,upquote=true,label={lst:extract_method_example}]
+ public static boolean isEmpty(final Object[] array) { 
+   return array == null || array.length == 0;
+ }
public static boolean isBlank(String str) {
-   if (str == null || str.length() == 0) {
-       return true;
-       }
-   return false;
+   return isEmpty(str); 
}
public static String camelToSplitName(String camelName, String split) {
-   if (camelName == null || camelName.length() == 0) {
+   if (isEmpty(camelName)) {
        return camelName;
    }
    ...
}
\end{lstlisting}

\noindent\emph{Coding style reformation (\#\foreachnumber{}, \foreachratio{}\%).}  \modifyhaibo{mention that different project has different requirements}.
\begin{lstlisting}[style=mystyle, escapechar=^,caption=Example of code style reformat,upquote=true,label={lst:condexample}]
- if (posts == null) {
-   posts = new ArrayList<Post>();
- }
+ if (posts == null) posts = new ArrayList<Post>();
\end{lstlisting}

\noindent\emph{Replace with annotations (\#\foreachnumber{}, \foreachratio{}\%).} \modifyhaibo{RefactoringMiner could not detect whether a segment of code is replace by semantic-preserving annotations}.
\begin{lstlisting}[style=mystyle, escapechar=^,caption=Example of  ``Replace with annotations'', upquote=true, label={lst:annotationexample}]
+ @Getter
+ @Setter
public class TestAppConfiguration {
  private String defaultName;
- public String getDefaultName() {
-       return defaultName;
- }
- public void setDefaultName(String defaultName) {
-       this.defaultName = defaultName;
- }
}
\end{lstlisting}

\noindent\emph{Use \texttt{foreach} for iteration (\#\foreachnumber{}, \foreachratio{}\%).}   In some program languages (e.g., Java, python, C++, C\#), \texttt{foreach} loop (or for each loop) is a control flow statement for traversing items in a collection and it is usually used in place of a standard \texttt{for} loop statement. It has the following syntax: \texttt{for each item in collection: do something to item}~\footnote{https://docs.oracle.com/javase/8/docs/technotes/guides/language/foreach.html}. Due to \texttt{foreach} loops usually maintain no explicit counter and directly fetch elements from a collection, this avoids potential off-by-one errors (a logic error involving the discrete equivalent of a boundary condition) and makes code simpler to read. During our manual analysis, we find out that developers usually simplify \texttt{for} statements to a collection via transforming other kinds of iterator to \texttt{foreach} when it comes to the iteration and operation of elements in the collection. Listing~\ref{lst:foreach_example} presents an example.
\begin{lstlisting}[style=mystyle, escapechar=^,caption=Example of using foreach for iteration,upquote=true,label={lst:foreach_example}]
- for (int symbol = 0; symbol < codeLensFromSym.length;++symbol) {
-  int codeLength=codeLensFromSym[symbol];
+ for (int codeLength : codeLensFromSym) {
    countsFromCodeLen[codeLength]++;
}
\end{lstlisting}

\noindent\emph{Merging imports (\#\foreachnumber{}, \foreachratio{}\%)}. Listing~\ref{lst:mergeexample} where several import statements under the same package are merged via the \texttt{java.util.*} expression.
\begin{lstlisting}[style=mystyle, escapechar=^,caption=Example of merging imports,upquote=true,label={lst:mergeexample}]
- import java.util.ArrayList;
- import java.util.Collections;
- import java.util.Iterator;
- import java.util.List;
- import java.util.Map;
- import java.util.WeakHashMap;
+ import java.util.*;
\end{lstlisting}

\noindent\emph{Code deletion (\#\foreachnumber{}, \foreachratio{}\%).} Delete unused imports, it is not considered as refactoring, but it can be done by tools.
\begin{lstlisting}[style=mystyle, escapechar=^,caption=Example of ``deleting code",upquote=true,label={lst:condexample}]
- private StringUtil() { //Unused
-   ... 
- }
\end{lstlisting}

\noindent\emph{Coding style reformation (\#\foreachnumber{}, \foreachratio{}\%).}  mention that different project has different requirements.
\begin{lstlisting}[style=mystyle, escapechar=^,caption=Example of ``code style reformat",upquote=true,label={lst:condexample}]
- if (posts == null) {
-   posts = new ArrayList<Post>();
- }
+ if (posts == null) posts = new ArrayList<Post>();
\end{lstlisting}

\noindent\emph{Merging imports (\#\foreachnumber{}, \foreachratio{}\%)}. Listing~\ref{lst:mergeexample} where several import statements under the same package are merged via the \texttt{java.util.*} expression.
\begin{lstlisting}[style=mystyle, escapechar=^,caption=Example of ``merging imports",upquote=true,label={lst:mergeexample}]
- import java.util.ArrayList;
- import java.util.Collections;
- import java.util.Iterator;
- import java.util.List;
- import java.util.Map;
- import java.util.WeakHashMap;
+ import java.util.*;
\end{lstlisting}

\noindent\textbf{Clean up code (\#\deletionnumber{}, \deletionratio{}\%).} The most frequent motivation is cleaning up code, which account for more than \deletionapproximateratio{}\% of studied PRs. Operations including removing redundant or unused code, getting rid of unused imports or cleaning up dead code blocks~\footnote{https://github.com/softicar/platform/pull/197}. These operation can be measured by checking for reduced code size.

\noindent\textbf{Readability (\#\readabilitynumber{}, \readabilityratio{}\%).} About one quarter of the studied PRs for simplifying programs originate from developers concerns about the readability of programs. %The readability of a program is related to its maintainability. 
Having readable code is essential for software maintenance as developers usually spend more time in maintaining code than writing code from scratch~\cite{boehm2001defect,buse2008metric,scalabrino2016improving}. We observe that developers usually improve readability by reformatting conditional statements, using APIs, inline temporary variables, and etc. For example,  developers use lambada expressions to simplify program by replacing anonymous methods, leading to shorter and cleaner program while preserving its functionality~\footnote{https://github.com/openhab/openhab-addons/pull/10941}.

\noindent\textbf{Complexity (\#\complexitynumber{}, \complexityratio{}\%).} Another common motivation is to reduce program complexity. Program complexity are related to project maintenance difficulty and introducing of the security vulnerabilities~\cite{lanning1994modeling,shin2008empirical}. Developers usually %would simplify program to 
reduce program complexity  by using Java polymorphism, replacing with equivalent APIs, use foreach for iteration and etc.

\noindent\textbf{Reusability (\#\reusabilitynumber{}, \reusabilityratio{}\%).} Developers may also simplify program to improve the reusability. Common operations include extracting common code blocks or some ``copy-paste code'' to reduce duplication and reuse existing code~\footnote{https://github.com/apache/commons-lang/pull/463}.
