# Supplementary material for: An Empirical Study of Refactoring Engine Bugs
Source: arXiv:2409.14610 source file (2024-09-22)
Supplement: Supplementary file 2 [file Supplement.tex]

\section*{Supplementary}
